# Supplementary material for: On discretisation drift and smoothness regularisation in neural network training
Source: arXiv:2310.14036 source file (2023-10-21)
Supplement: Supplementary file 1 [file introduction_supplementary.tex]

\chapter{Optimisation Background Supplementary}

\section{Stability analysis derivation}

\label{sec:stability_analysis_derivation}

We now provide a justification for the stability analysis result we provided in Section~\ref{sec:stability_analysis_overview}. We start with a linearisation argument: consider a neighbourhood $\mathcal{U}$ such that $\vtheta^* \in \mathcal{U}$ and the linear approximation of $f(\vx) = f(\vtheta^*) + \jacthetaf(\vtheta^*) (\vtheta - \vtheta^*)=  \jacthetaf(\vtheta^*) (\vtheta - \vtheta^*)$ is exact. We note that this is not a formal argument, for a rigurous proof we rely on the Hartman–Grobman theorem~\citep{grobman,hartman1960lemma}. 

We then have:
\begin{align}
 \dot{\vtheta} = f(\vtheta) = \jacthetaf(\vtheta^*) (\vtheta - \vtheta^*)
\end{align}

leading to 
\begin{align}
 \dot{(\vtheta - \vtheta^*)} = f(\vtheta) = \jacthetaf(\vtheta^*) (\vtheta - \vtheta^*)
\end{align}

which is a linear system with the solution:
\begin{align}
\vtheta(t) = \vtheta^* + e^{\jacthetaf(\vtheta^*)t} (\vtheta(0) - \vtheta^*)
\end{align}

Thus to show exponential asymptotic convergence, we need to show that $\lim_{t \rightarrow \infty}  e^{\jacthetaf(\vtheta^*)t} (\vtheta(0) - \vtheta^*) = 0$ and it does so at an exponential rate. To do so, we have to use the assumption that  $\jacthetaf(\vtheta^*)$ only has eigenvalues with negative real part.
Since $\jacthetaf(\vtheta^*)$ need not be symmetric, its eigenvalues can be complex. We then rely on the Jordan normal form of $\jacthetaf(\vtheta^*)$ and write:
\begin{align}
\jacthetaf(\vtheta^*) = P^{-1} J P
\end{align}

where $J$ is a block diagonal matrix 
\begin{align}
J = \begin{bmatrix}
{J_0} & \hdots & 0 & 0\\
0 & {J_1} & \hdots & 0 \\
\vdots &  &  & \vdots \\
 0 & \hdots & 0 & {J_{m}}\\
\end{bmatrix} 
\end{align}
Each block $J_k$ corresponds to a unique eigenvalue $\lambda_k$ with duplicity $n_k$, with $J_k \in \mathbb{C}^{n_k, n_k}$ where
\begin{align}
 J_{k} = \lambda_k I_{n_k} + Z_{n_k}
\end{align}

where $ I_{n_k}$ is the identity matrix of dimension $n_k$ and $Z_{n_k}$ is a matrix with all $0$s apart from one off diagonal:
\begin{align}
Z_{n_k} = \begin{bmatrix}
0 & 1&  \hdots & 0 & 0 \\
0 & 0&  1 & \hdots & 0 \\
\vdots & \vdots& \ddots & \ddots &  \vdots\\
0 & 0 & 0 & \hdots & 1 \\
0 & 0 & 0 & 0 & 0
\end{bmatrix}
\label{eq:z_structure}
\end{align}

We have that
\begin{align}
e^{\jacthetaf(\vtheta^*) t} &= e^{P^{-1} J P t} = \sum_{i=0}^{\infty} \frac{1}{i!} (P^{-1} Jt P)^i \\ 
                                 &=  \sum_{i=0}^{\infty} \frac{1}{i!} P^{-1} (Jt)^i P= P^{-1} \left(\sum_{i=0}^{\infty} \frac{1}{i!} (Jt)^i\right) P = P^{-1}e^{Jt}  P 
\end{align}

and thus
\begin{align}
 \norm{e^{\jacthetaf(\vtheta^*)t} (\vtheta(0) - \vtheta^*)}_F &\le \norm{{P^{-1}e^{Jt}  P }}_F \norm{(\vtheta(0) - \vtheta^*)}_F \\
 &\le \norm{e^{Jt}}_F\norm{P^{-1}}_F \norm{P}_F \norm{(\vtheta(0) - \vtheta^*)}_F
 \label{eq:stability_analysis_norm}
\end{align}

We are thus left with the task of bounding $\norm{e^{Jt}}$. Since $J$ is a block-diagonal matrix and thus its structure is preserved under addition and multiplication, if we use the Taylor expansion of the exponential we can write:
\begin{align}
e^{Jt} = \begin{bmatrix}
e^{J_0 t} & \hdots & 0 & 0\\
0 & e^{J_1 t} & \hdots & 0 \\
\vdots &  &  & \vdots \\
 0 & \hdots & 0 & e^{J_{m} t}\\
\end{bmatrix} 
\end{align}

If we consider the Frobenius norm, we have
\begin{align}
\norm{e^{J t}}^2_F = \sum_{i=1}^{m} \norm{e^{J_m t} }^2_F \le m \norm{e^{J_k t}}^2_F
\label{eq:e_j_bound}
\end{align}

where $J_k$ is the block with the maximum Frobenius norm in $J$. Now using the form of $J_k$ we have:

\begin{align}
\norm{e^{J_k t}}_F = \norm{e ^{\lambda_k t I + t Z_{n_k}}}_F = \norm{e ^{t \lambda_k I}_F e^ {t Z_{n_k}}}_F
 \le \norm{e ^{t \lambda_k I}}_F \norm{e^{ t Z_{n_k}}}_F
\end{align}

Using the form of $Z_{n_k}$ in Eq~\eqref{eq:z_structure} we have that
\begin{align}
e^{t Z_{n_k}} = \sum_{i=0}^{\infty} \frac{1}{i!}{(t Z_{n_k})}^i = \sum_{i=0}^{n_k} \frac{1}{i!}{ (t Z_{n_k})}^i
\end{align}

since ${Z_{n_k}}^i =0$ for $i \ge {n_k}$. We thus can treat $\norm{e^ {Z_{n_k}}}_F$ which we denote as $C$. We then have:
\begin{align}
\norm{e^{J_k t} }_F \le C \norm{e ^{t \lambda_k I}}_F
\label{eq:j_k_bound}
\end{align}{}

If we use the assumption that $\lambda_k$ has negative real part we have $\lambda_k = -x + i y$ with $x > 0$ and:
\begin{align}
\norm{e ^{t \lambda_k I}}_F = \sqrt{n_k} \norm{e ^{t \lambda_k}}_F  = \sqrt{n_k} \norm{e ^{-x  t+ i t y}}_F \le  \sqrt{n_k} \norm{e ^{-x t}}_F \norm{e ^{i t y}}_F 
\label{eq:lambda_k_bound}
\end{align}

Thus from Eqs~\eqref{eq:j_k_bound} and~\eqref{eq:lambda_k_bound} we have:
\begin{align}
\norm{e^{t J_k}}_F \le C n_k e ^{-t x}
\end{align}

with $x = \Re(\lambda_k)$. Replacing back in Eq~\eqref{eq:e_j_bound} we have:
\begin{align}
\norm{e^{J t}}_F \le \sqrt{m n_k} C e ^{-t x}
\end{align}

Replacing back in Eq~\eqref{eq:stability_analysis_norm} leads to:
\begin{align}
 \norm{e^{\jacthetaf(\vtheta^*)t} (\vtheta(0) - \vtheta^*)}_F 
 &\le \norm{e^{t J} }_F\norm{P^{-1}}_F \norm{P}_F \norm{(\vtheta(0) - \vtheta^*)}_F \\
 &\le  \sqrt{m n_k} C e ^{-t x} \norm{P^{-1}}_F \norm{P}_F \norm{(\vtheta(0) - \vtheta^*)}_F \\
 &\le K e ^{- t x} \norm{(\vtheta(0) - \vtheta^*)}_F
\end{align}

with $x > 0$ which concludes the proof.

\section{Nash equilibria and stable fixed points in games}

\label{app:sup_games_nash_equilibria}

We now discuss the differences between Nash equilibria and local stability in games. The continuous-time flow of the form: 
\begin{align}
\dot{\vphi} = -\nabla_{\vphi} E_{\vphi}  \\
\dot{\vtheta} = -\nabla_{\vtheta} E_{\vtheta} 
\end{align}

is attracted to equilibria for which the full game Hessian 
\begin{align}
\left[ 
\begin{array}{c|c} 
  \nabla_{\vphi}^2 E_{\vphi} & \nabla_{\vtheta}\nabla_{\vphi} E_{\vphi} \\ 
  \hline 
  \nabla_{\vphi}\nabla_{\vtheta} E_{\vtheta} & \nabla_{\vtheta}^2 E_{\vtheta}
\end{array} 
\right] 
\end{align}

evaluated at $(\vphi^*, \vtheta^*)$ has only eigenvalues with positive real part. In the most general setting this condition is different than that of a Nash equilibrium, which requires that $\nabla_{\vphi}^2 E_{\vphi}$ and $ \nabla_{\vtheta}^2 E_{\vtheta}$ are positive definite.
Without making assumpitons about the structure of the game, one cannot make any assertions about the relationship between Nash equilibria and stable fixed points in games. 
To see why, consider the matrix
\begin{align}
\left[ 
\begin{array}{c|c} 
 1 & 1\\ 
  \hline 
  2 & 1
\end{array} 
\right] 
\end{align}

which has positive definite diagonal blocks, but its eigenvalues do not only have positive real part since they are $1 \pm \sqrt 2$ and $1 - \sqrt 2$ is negative. We have thus found a matrix that could correspond to a Nash equilibruim, but would not be locally attractive.

Conversely, we can find a matrix which has diagonal blocks which are not positive definite, but which only has eigenvalues with negative real part. Consider
\begin{align}
\left[ 
\begin{array}{c|c} 
 -1 & 1\\ 
  \hline 
  -8 & 5
\end{array} 
\right] 
\end{align}

with eigenvalues $1, 3$, both with positive real part but the upper diagonal block does not satisfy this property and thus this cannot be the Hessian of a Nash equilibrium.

\textbf{A note on zero-sum games}. If we consider zero-sum games with $E_{\vphi} = - E_{\vtheta} = E$

\begin{align}
\left[ 
\begin{array}{c|c} 
  \nabla_{\vphi}^2 E & \nabla_{\vtheta}\nabla_{\vphi} E\\
  \hline 
  - \nabla_{\vphi}\nabla_{\vtheta} E & - \nabla_{\vtheta}^2 E
\end{array} 
\right] 
\end{align}

Consider $\vphi^*, \vtheta^*$ a Nash equilibrium, i.e. $\nabla_{\vphi}^2 E $ is positive definite and so is $- \nabla_{\vtheta}^2 E$.

\begin{align}
&[\vx, \vy]
\left[
\begin{array}{c|c} 
  \nabla_{\vphi}^2 E & \nabla_{\vtheta}\nabla_{\vphi} E\\
  \hline 
  - \nabla_{\vphi}\nabla_{\vtheta} E & - \nabla_{\vtheta}^2 E
\end{array} 
\right] \left[ \begin{array}{c} 
  \vx \\
  \vy
\end{array} 
\right] \\
&= 
\vx^T \nabla_{\vphi}^2 E \vx - \vy^T \nabla_{\vphi}\nabla_{\vtheta} E \vx + \vx^T \nabla_{\vtheta}\nabla_{\vphi} E \vy - \vy^T \nabla_{\vtheta}^2 E \vy \\
&=\vx^T \nabla_{\vphi}^2 E \vx - \vy^T \nabla_{\vtheta}^2 E \vy < 0
\end{align}

where we used that 
\begin{align}\vy^T \nabla_{\vphi}\nabla_{\vtheta} E \vx = (\vy^T \nabla_{\vphi}\nabla_{\vtheta} E \vx)^T = \vx^T \nabla_{\vphi}\nabla_{\vtheta} E^T \vy = \vx^T \nabla_{\vtheta}\nabla_{\vphi} E \vy
\end{align}

This allows us to observe that if a Hessian matrix is block antisymmetric, i.e $\nabla_{\vtheta}\nabla_{\vphi} E = - \nabla_{\vphi}\nabla_{\vtheta} E^T$ then a Nash equilibrium is locally attractive. We note that the reverse does not hold, as being locally attractive in this case is a weaker condition than that of a Nash equilibrium.

A further discussion about types of equilibria, specifically in the GANs is provided by \citep{berard2019closer}.
